# Supplementary material for: Learning Representations for Pixel-based Control: What Matters and Why?
Source: arXiv:2111.07775 source file (2021-11-15)
Supplement: Supplementary file 1 [file appendix.tex]

\appendix

% \clearpage
% \bibliography{iclr2022_conference}
% \bibliographystyle{iclr2022_conference}

% \end{document}
